# Supplementary material for: Stop&Hop: Early Classification of Irregular Time Series
Source: arXiv:2208.09795 source file (2022-08-21)
Supplement: Supplementary file 1 [file 8_appendix.tex]

First, thank you, the reviewer, for your service to us and our community. You made it to our supplement, so we look forward to improving our work given your thoughtful feedback.

\section{Private Code-Preview}
We have written a working example in Python and present you with private early access, uploaded as a zip folder along with our submission. %\footnote{\url{https://github.com/DoubleBlindSubmissions/StopHopPrivatePreview}}
Please peruse our code; we added documentation with you in mind.
We kindly ask that you refrain from sharing our code while our work is unpublished.

% \footnote{\url{https://github.com/DoubleBlindSubmissions/StopHopPrivatePreview}}

To ease your onboarding into our framework, we \textit{pre-computed} a set of irregular time series prefix embeddings for the \textsc{PhysioNet} dataset, neatly bundled into two PyTorch loaders (training and testing).
With PyTorch loaders in hand, you can avoid training any continuous-time RNNs---it is reproducible, but slow.
While pre-computing makes our system easier to digest, it loses the capacity to compute hidden states at \textit{any} continuous value, even though \method takes real-valued hops in the continuous timeline.
To reconcile this difference and for simplicity, we round \method's halting times to the nearest embeddings for this private preview.
For example, if \method were to hop for 1.7 minutes, but the nearest embedding is actually 2 minutes away, we just use the 2-minute-away embedding and pretend that \method chose to hop for 2 minutes during optimization.
This is, of course, a simpler version of our proposed method.
In a real application, it is entirely feasible---recommended, even---to do everything in continuous-time: Let \method pick a hop-size, then compute a prefix embedding at exactly that time. The fully-continuous version is simply slower and requires training the RNN concurrently, which hinders our purpose: providing a palatable preview of our code.

\section{\method Inference Algorithm}
To ensure \method is intuitive, accessible, and extensible, we also provide Algorithm \ref{alg:alg}, a high-level description of \method at inference time.
The input $X$ is, of course, not entirely available when the algorithm starts. Future values are only observed when $\pi_\text{hop}$ decides to hop forwards. Further, the value $T$, the maximum allowable time for the algorithm to run, is up to the user. In practice, $T$ can be set to known or predictable time series lengths, or left large as an infinite horizon. It may even be possible to learn $T$ as it is certainly reasonable that the best $T$ differ by time series.

% \begin{figure}[H]
\begin{algorithm}[b!]
\caption{Inference with \method}\label{alg:alg}
\KwIn{$X$}
\KwResult{$\hat{y}, \tau$}
$t^\prime \gets 0$\\
\While{$t^\prime < T$}{
    $h_{t^\prime} \gets \mathcal{R}_\theta(X_{\leq t^\prime})$\\
    $\hat{y}_{t^\prime} \gets \mathcal{C}_\theta(X_{\leq t^\prime})$\\
    $\text{Stop} \gets \pi_\text{stop}(h_{t^\prime}, \hat{y}_{t^\prime})$ \Comment*[r]{$\text{Stop} \in \{0, 1\}$}
    \eIf{$\text{Stop} = 1$ or $t^\prime \geq T$}{
        $\hat{y} \gets y_{t^\prime}$\\
        $\tau \gets \min(t^\prime, T)$\\
    % }{\If{$\text{Stop} = 0$}{
    }{
        $\Delta t \gets \pi_\text{hop}(h_{t^\prime}, \hat{y}_{t^\prime})$  \Comment*[r]{$\Delta t \in [0, \max(T, T_\text{max})]$}
        $t^\prime \peq \Delta t$
        }
    }
\end{algorithm}
% \end{figure}

% \begin{figure}[t]
% \begin{algorithm}[h]
% \begin{algorithmic}
% \SetAlgoLined
% \KwResult{Class prediction $\hat{y}$, Halting time $\tau$}
%     $t^\prime = 0$\;
%     $a_{t^\prime} = 0$\;
%     $h_{t^\prime} = 0 \in \mathbb{R}^{D}$\;\\
%     \While{$a_{t^\prime} \neq 1$ and $t^\prime \leq T_\text{max}$}{
%         $h_{t^\prime} = \text{ITSPrefixEncoder}(X, t^\prime)$\;\\
%         $a_{t^\prime} = \text{HaltingPolicyNetwork}(h_{t^\prime})$\;\\
%     \If{$a_{t^\prime} \neq 1$}{
%         $\Delta t = \text{Hop}(h_{t^\prime}, t^\prime)$\;
%         $t^\prime \mathrel{+}= \Delta t$\;
%     }
%     }
%     $\hat{y} = \text{PrefixClassifier}(h_{t^\prime})$\;
%     $\tau = t^\prime$\;
%     \caption{Inference with \method}\label{alg:general}
%     \end{algorithmic}
% \end{algorithm}
% \end{figure}

\section{Ethical Considerations}
Our work facilitates decision making given partial temporal information.
This can naturally lead to misclassifications, which are more or less dangerous depending on the task and specifics of a given time series.
For example, an early \textit{Cancer} prediction may cause undue stress and financial burden to a patient if it turns out to be wrong.
Still, the cost of risking a false positive must be balanced with the cost of delaying predictions, which itself may have negative impacts.
We believe not that early classifiers \textit{suffer from or introduce} this trade-off, but that they \textit{embrace reality}---the trade-off is real in practice, regardless of the algorithm.
Standard classifiers, for instance, ignore prediction timing, so they always pick one side of the trade-off!
% We pose that non-early classifiers already incur this cost naturally as they already ignore prediction timing, generating all of their predictions concurrently without learning \textit{when} to make a prediction.

\section{Expanded Dataset Descriptions}
Two of our datasets, \textsc{Running} and \textsc{Walking} are new and will be released to the community.

While the datasets themselves are new, the way we create them is well-founded and thoroughly described in a concurrent in-submission paper.
At risk of cross-pollination, we describe the datasets here, too.
If \method is accepted first, we will release the datasets with this work as we believe the community will benefit from access to them and will expand on this generation direction.

\textsc{ExtraSensory} is a human activity recognition dataset: Participants downloaded mobile applications that logged their movement (e.g., accelerometer or gyroscope), then recorded what activities they did when.
These \textbf{data were collected in the wild}, so participants were left to their own devices for the duration of the study with no prescribed behavior.

\begin{figure*}[t]
    \centering
    \begin{subfigure}{0.32\linewidth}
        \includegraphics[width=\textwidth]{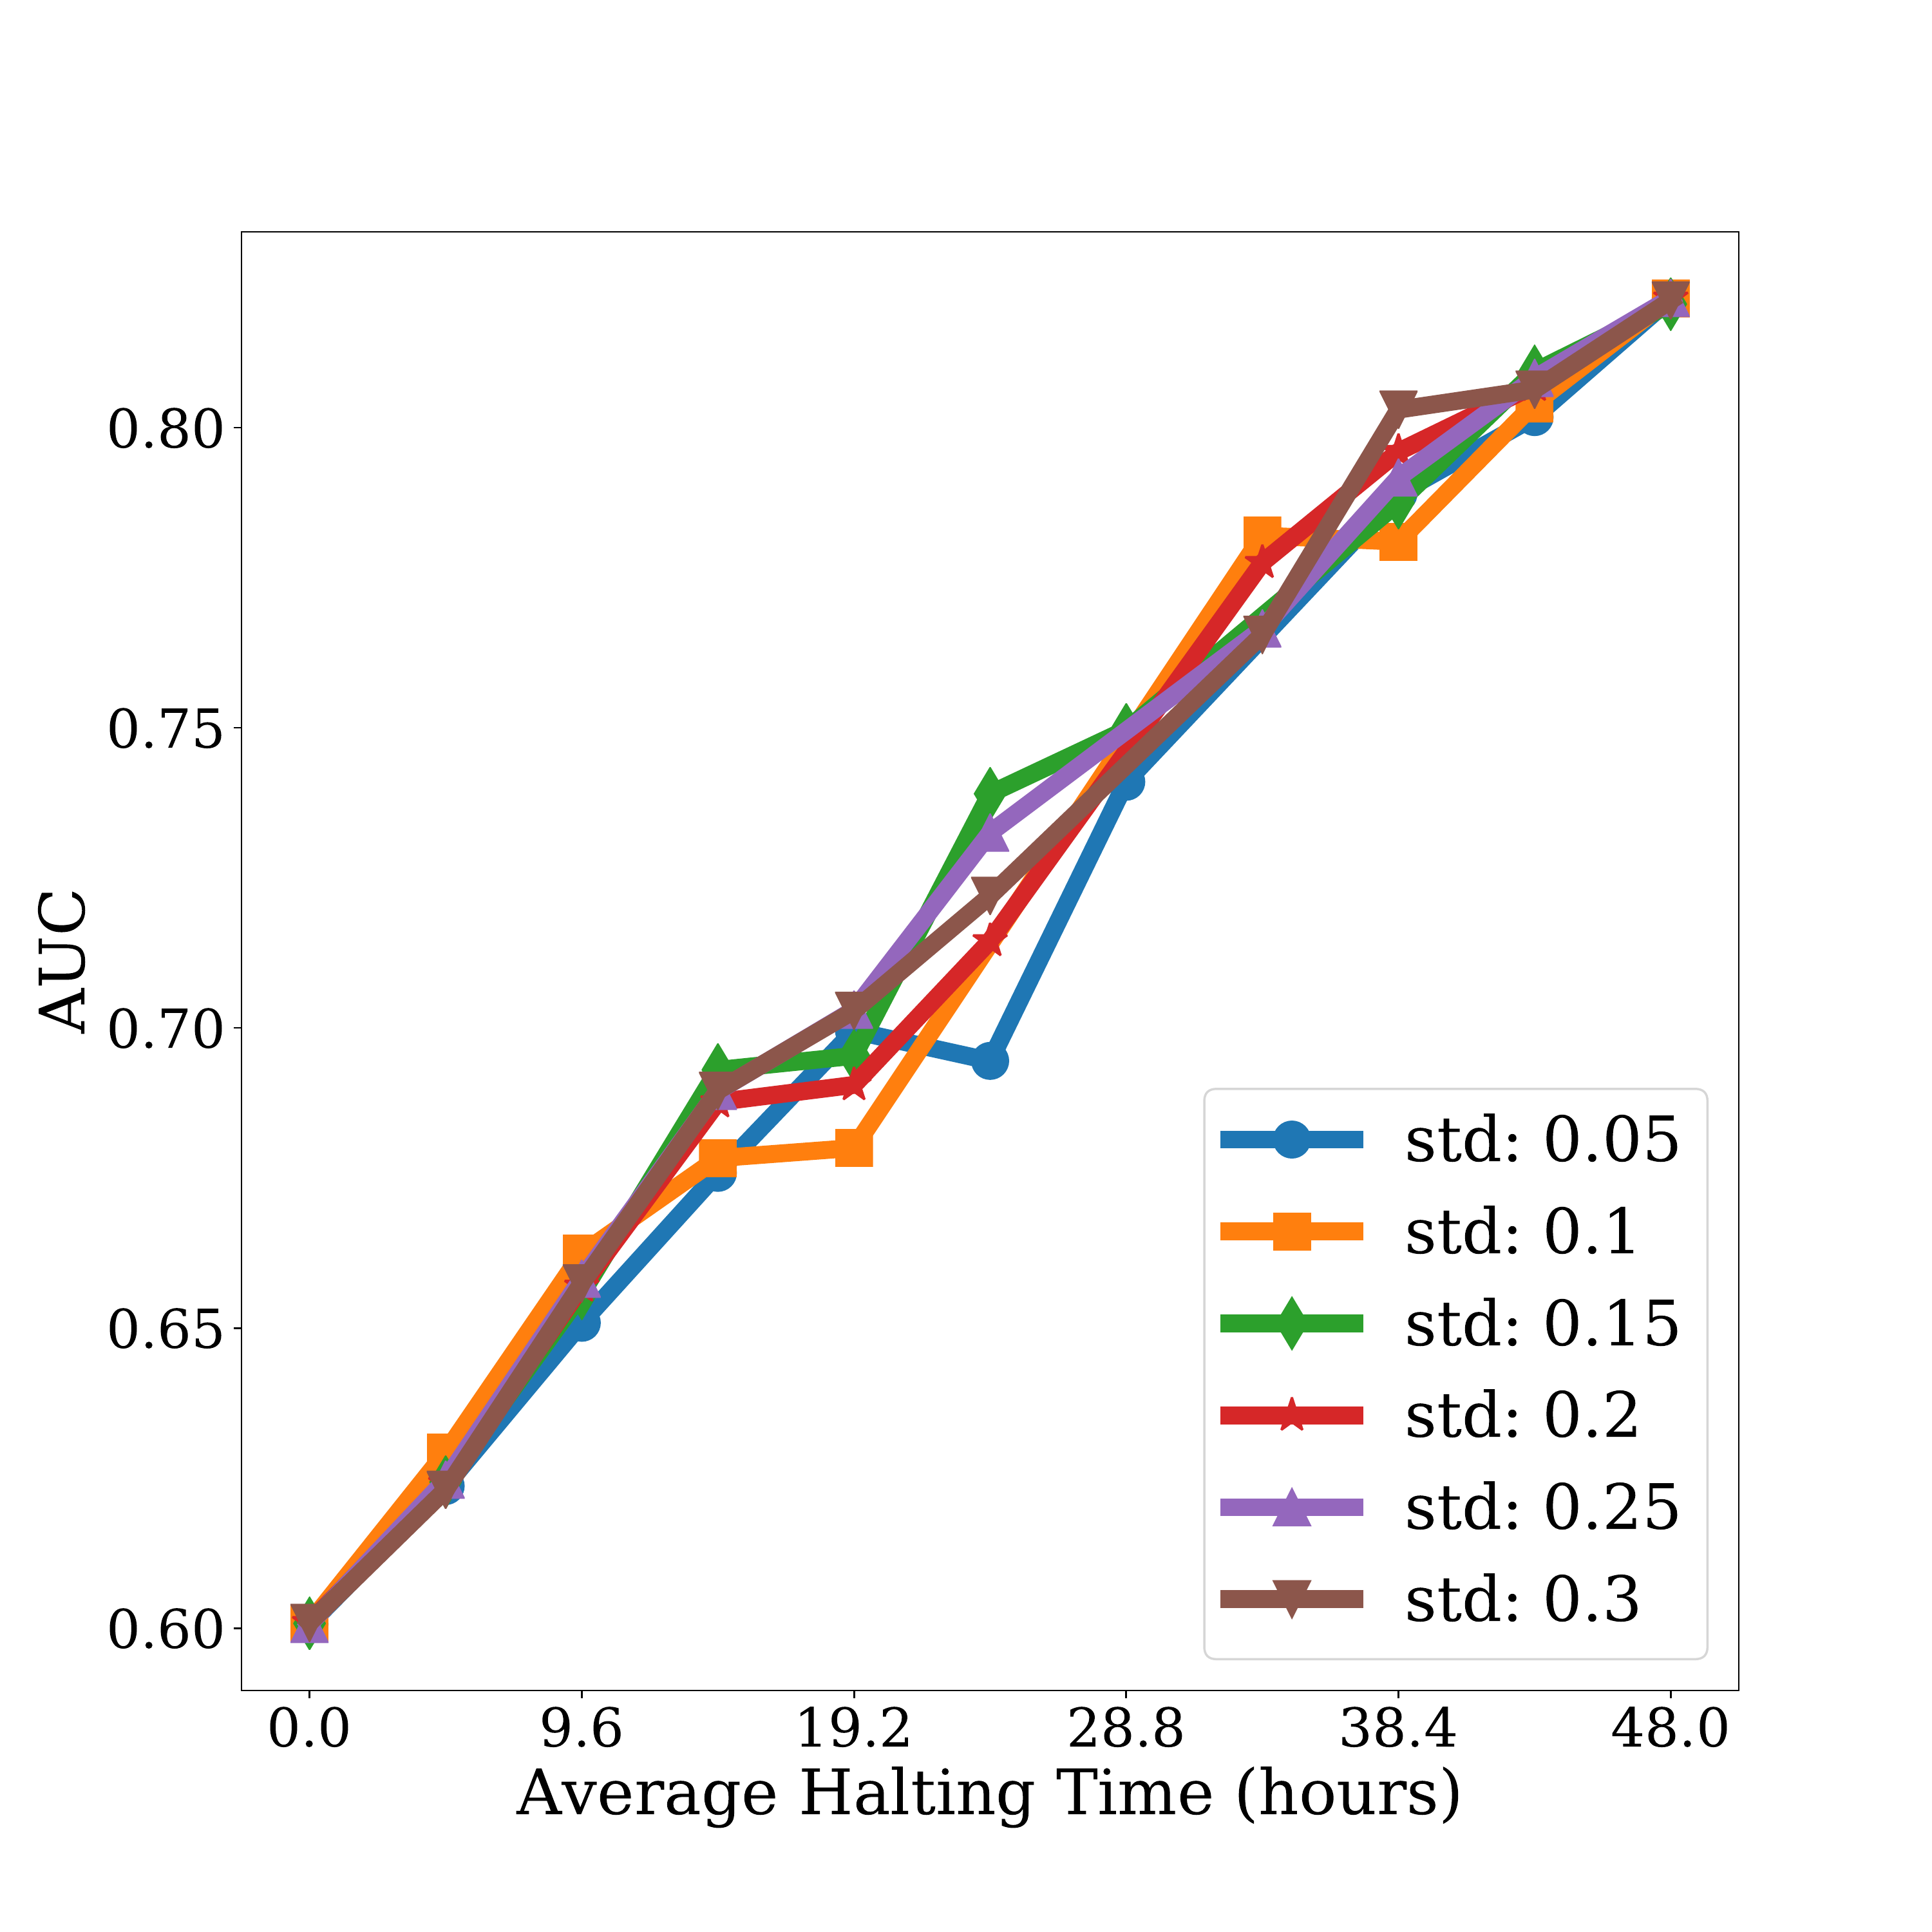}
        \vspace{-5mm}
        \caption{\textsc{PhysioNet}}
    \end{subfigure}
    \begin{subfigure}{0.32\linewidth}
        \includegraphics[width=\textwidth]{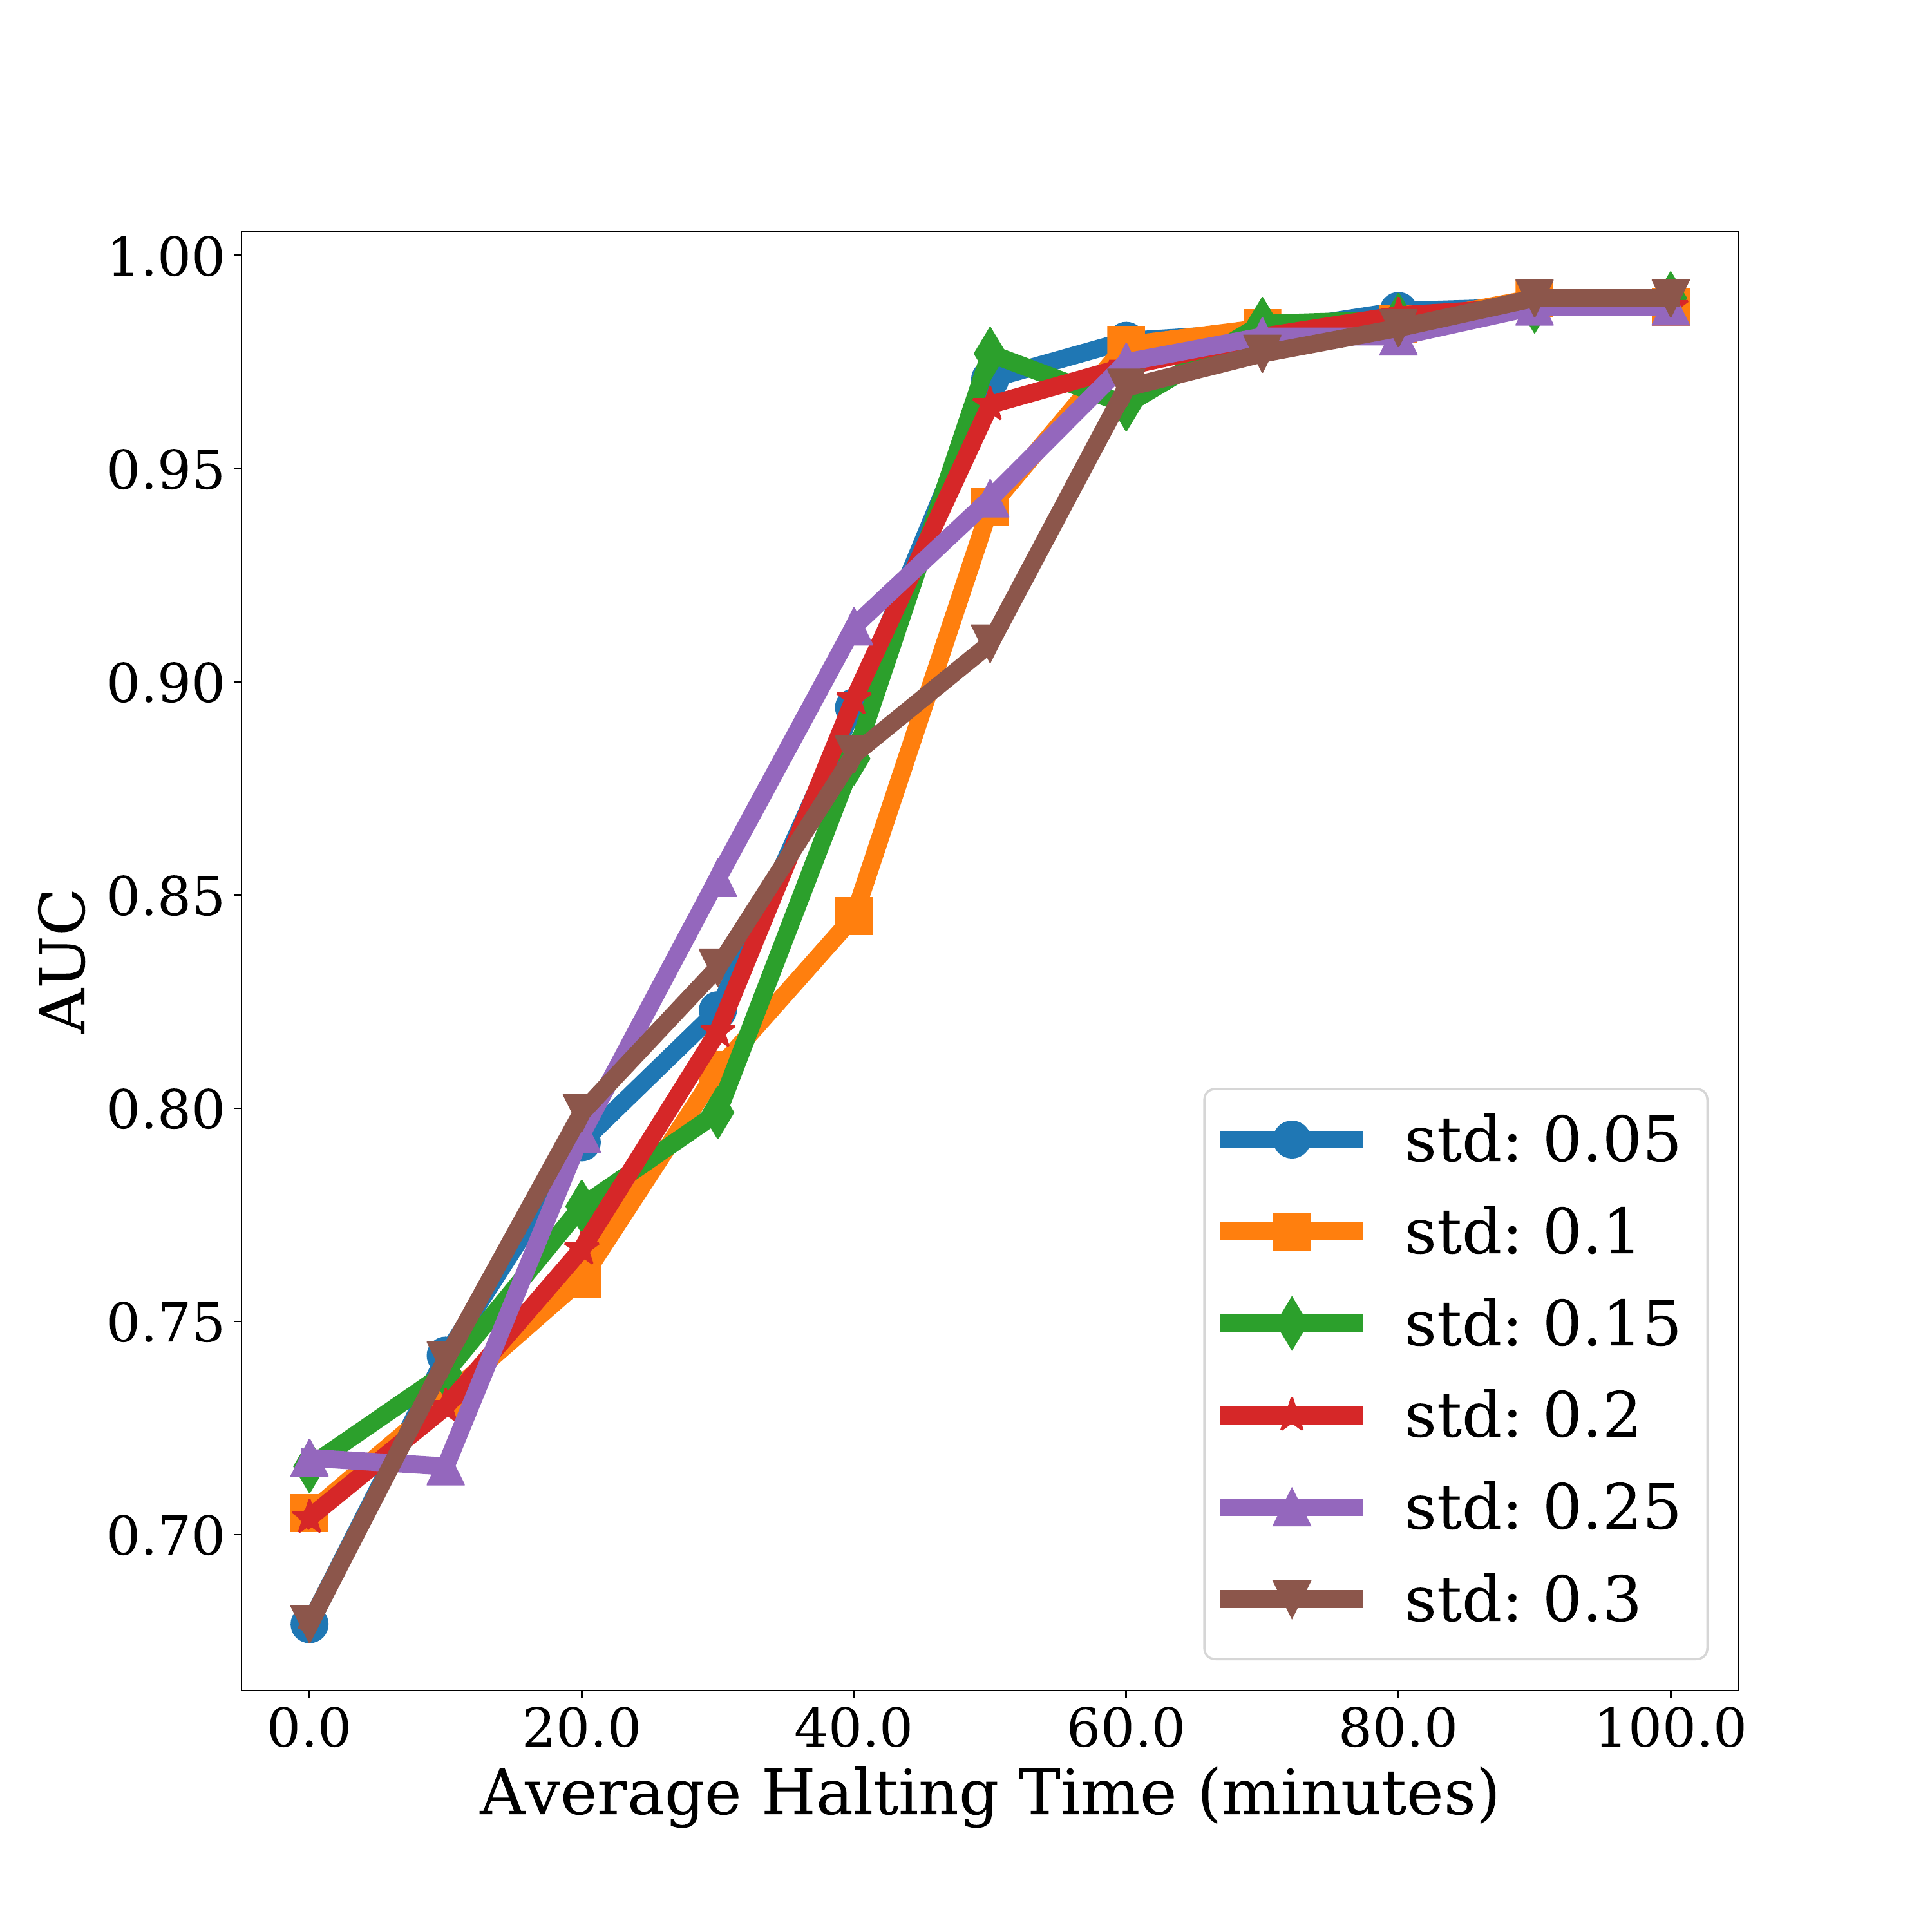}
        \vspace{-5mm}
        \caption{\textsc{ExtraSensory Running}}
    \end{subfigure}
    \vspace{2mm}
    \begin{subfigure}{0.32\linewidth}
        \includegraphics[width=\textwidth]{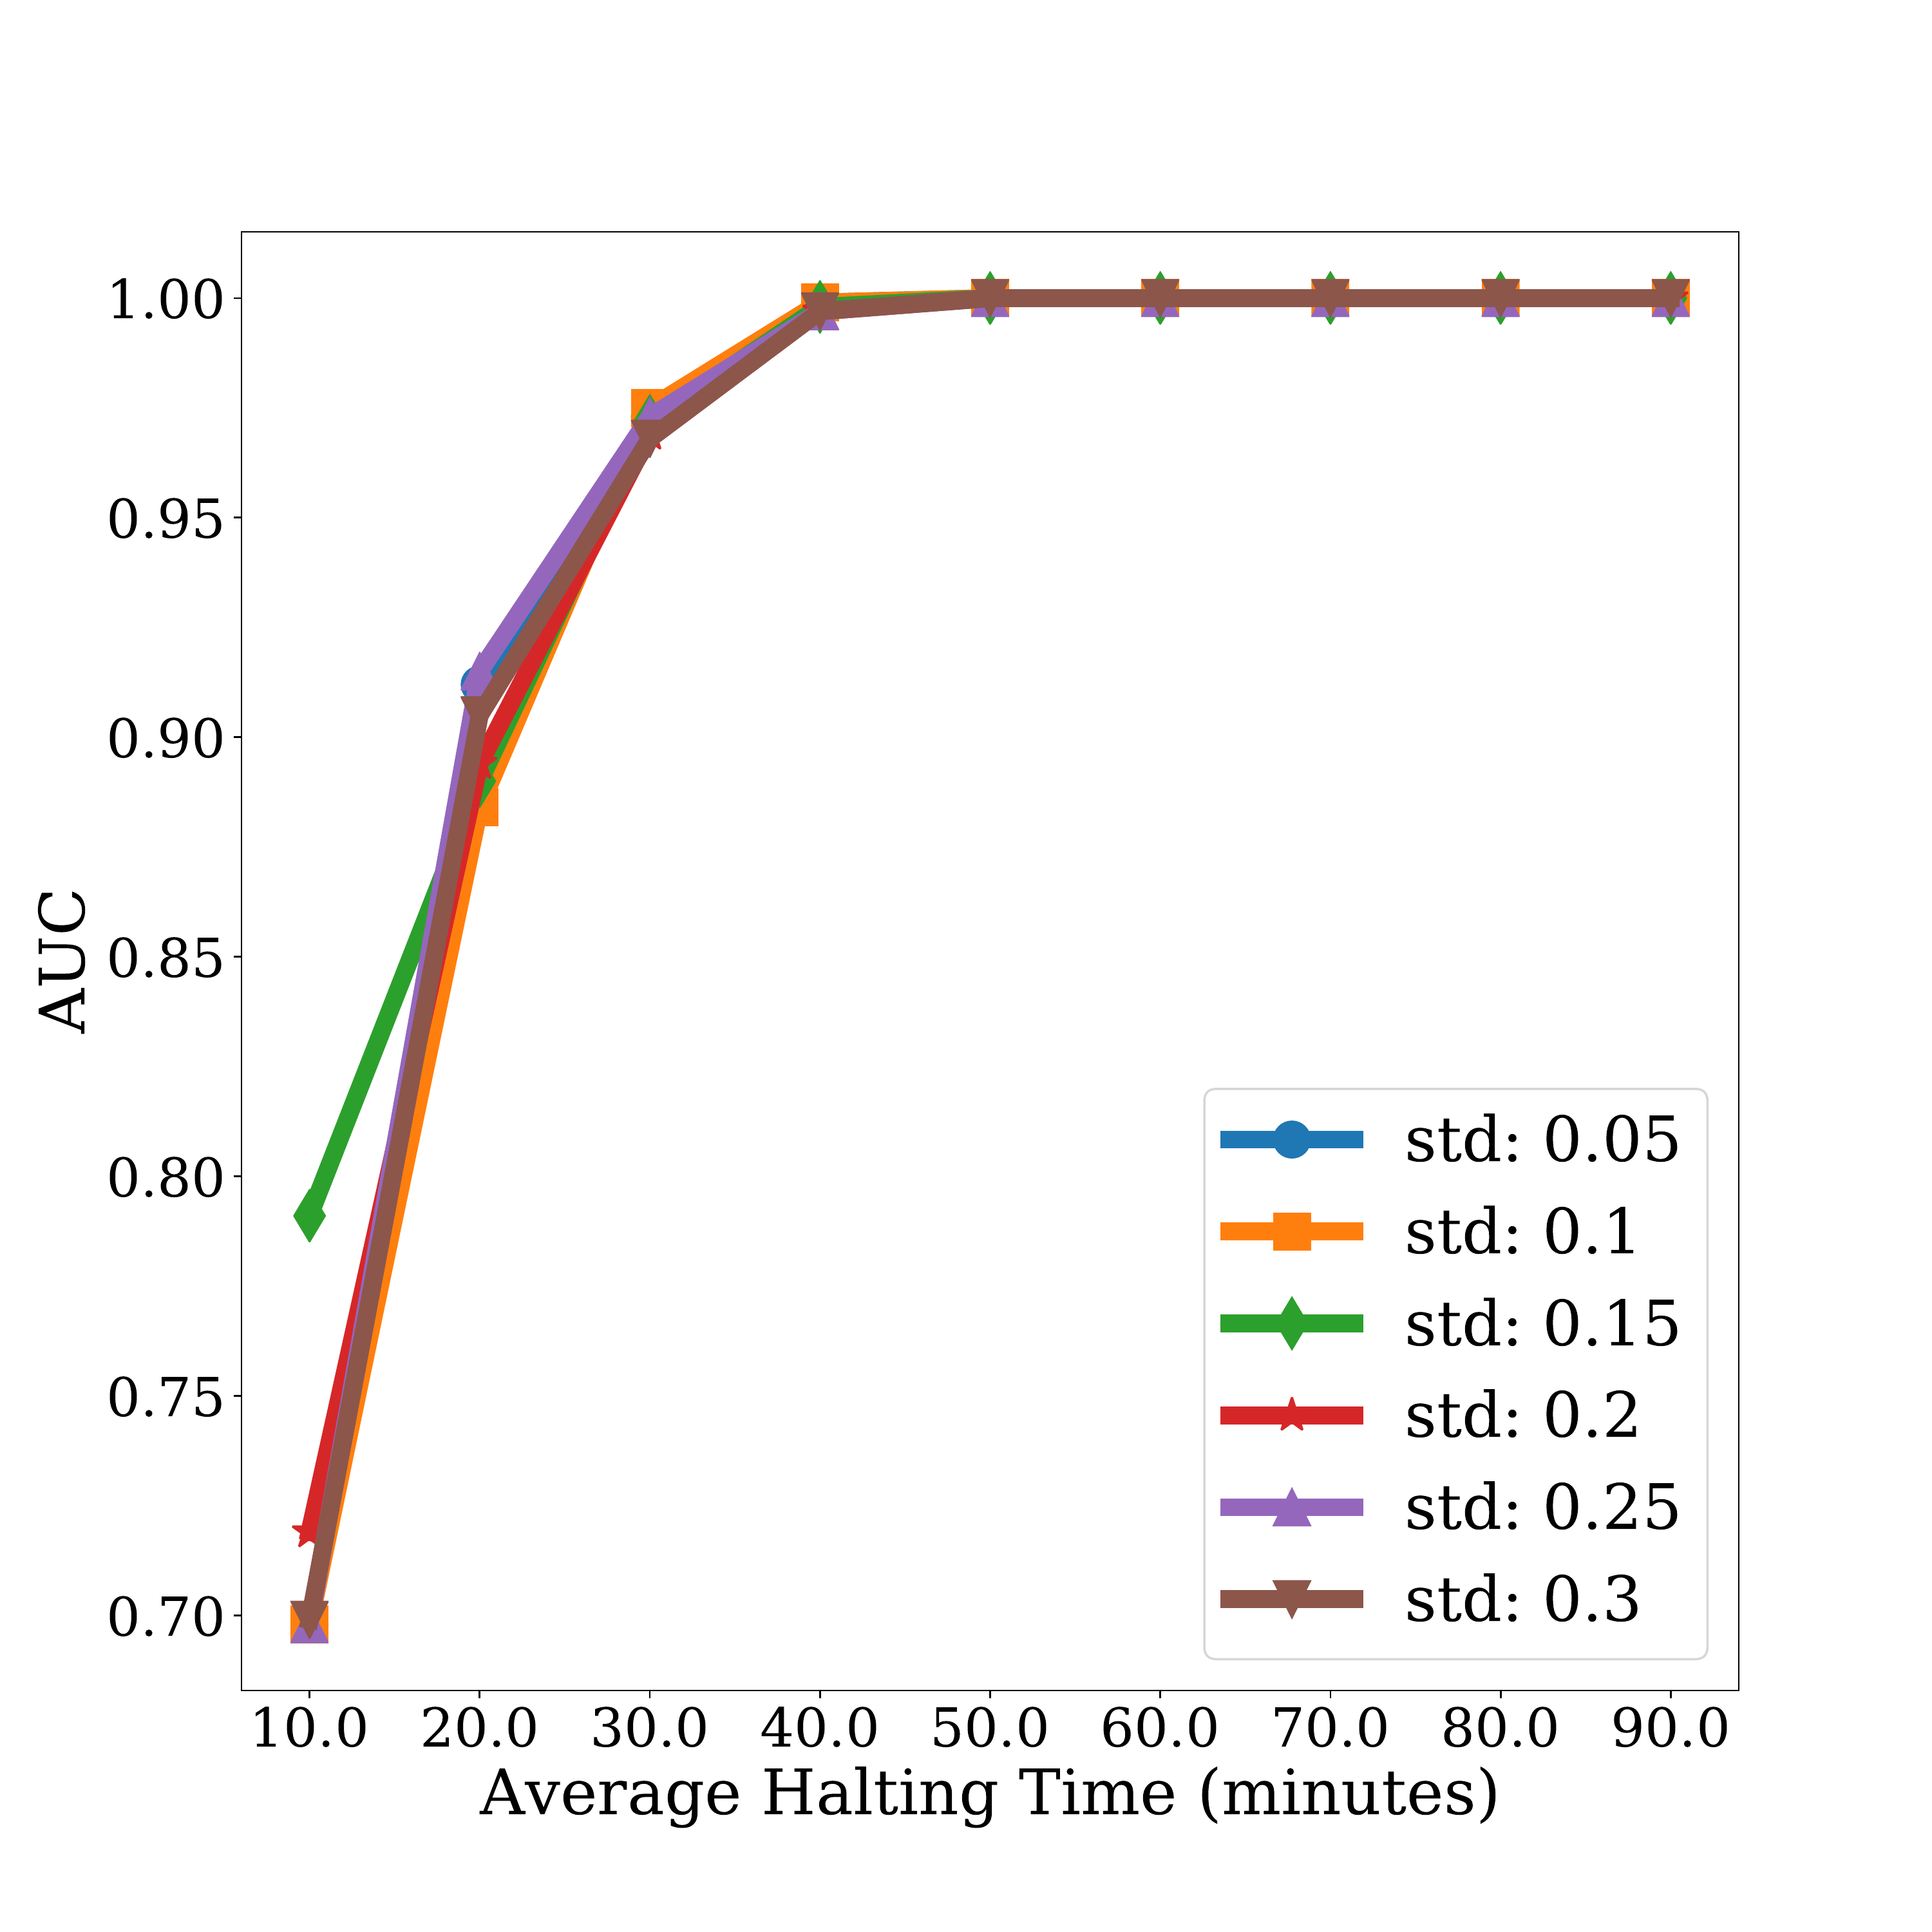}
        \vspace{-5mm}
        \caption{\textsc{ExtraSensory Walking}}
    \end{subfigure}
    \vspace{2mm}

    \vspace{-3mm}
    \caption{Effect of Hopping Policy's standard deviation (one of \method's hyperparameters) on the earliness accuracy trade-off curves. As the curves are similar to one another, \method is generally robust to selecting the standard deviation, though tuning per dataset can still be valuable.
    }
    \label{fig:std_hyper}
\end{figure*}

The \textsc{ExtraSensory} team collected data from 60 people over X days, creating a massive amount of smartphone data.
For this study, we extract only the raw accelerometer measures in the X, Y, and Z directions.
In line with prior work that successfully detects human activity from smartphone sensor data, we use only one person's accelerometer data for each of two activities: Walking and Running.
We choose the users who performed these activities the most.
Using one person at a time is a reasonable choice; activity signatures are often unique and entirely unrelated from anyone else's.
This is why human activity recognition work usually trains one model per participant instead of learning one model for all.

These specific data are not naturally irregular, but there are many cases where they can be.
For instance, many studies on wearable device data have found that participants cannot consistently provide reliable data: they leave their phone on the table, they forget to upload their activities, they stop participating altogether, etc.
These all create irregularity in real data environments, and for wearable devices in particular, especially moving beyond smartphones to smart rings and watches, these problems only grow \cite{goodday2021alternative}.

Knowing that irregularity is already common wearable sensor data, we introduce an alternative, realistic paradigm for creating irregular smartphone data: simulating a \textit{listening probe}.
Listening probes monitor ongoing time series data and chooses when to record the values.
By collecting only \textit{some} of the data, battery life is extended and memory is saved.
However, the resulting time series are irregular.
Listening probes can be implemented on different sensors, but since we are using accelerometer data, we simulate a listening probe on the accelerometer.
We use a simple \textit{threshold}-based listening probe: if the accelerometer values increase above a threshold, the data are collected.
So when a person moves their phone quickly, we get their data.
Alternatives listening probes exist.
We could record statistics about ongoing time series and detect outliers, for instance.
Our codebase introduces this new way to study irregular time series.
In summary, simulating listening probes on human activity recognition data lets us study new types of irregular series; sources of irregularity vary and should be considered differently.

To generate \textsc{Running} and \textsc{Walking} we threshold the norm of the 3-dimensional raw accelerometer data at 0.001: if the norm goes over 0.001, the data are collected.
For the users who performed their activities the most, we then chunk their data into non-overlapping 100-minute windows of time series data. To avoid cross-contamination between training and testing sets, we do the training, validation, and testing splits \textit{in time}: we train on early data and test on later data.

\section{Extended Implementation Details}
For each method, we use a batch size of 32 and grid search for a learning rate (options: $\{1e^{-2}, 1e^{-3}, 1e^{-4}\}$) and weight decay for L2 regularization (options: $\{1e^{-3}, 1e^{-4}, 1e^{-5}\}$) using our validation data.
The validation data is a random 10\% of the training dataset and we repeat this random splitting five times.
In our experiments, since we use a GRU-D \cite{che2018recurrent} to compute prefix embeddings, its hidden state should be updated in between hop sizes. For simplicity, we only update the embeddings when real data are observed per the baselines, though \method's final Stop time may be between observations.

\section{Extended Hyperparameter Study}
We also consider the standard deviation $\sigma$ of the hop policy $\pi_\text{hop}$, which controls for how long to wait before trying to stop again. As $\sigma$ increases, so does the variance in chosen hop sizes. Interestingly, we find that \method's performance is largely robust to changing $\sigma$, as shown in Figure \ref{fig:std_hyper}. Still, varying $\sigma$ seems to have some impact and we recommend tuning it according to the task at hand. $\sigma$ also determines to what degree $\pi_\text{hop}$ directly controls the sampled hop size. As $\sigma$ grows, $\pi_\text{hop}$ has less direct control, which can improve exploration and regularize the log probabilities of the chosen actions during training.

\vfill
